# Supplementary material for: History repeats Itself: A Baseline for Temporal Knowledge Graph Forecasting
Source: arXiv:2404.16726 source file (2024-04-29)
Supplement: Supplementary file 1 [file results_supplementary.tex]

% All recurrency baselines run on CPU; we use an Intel Xeon Silver (2.10GHz) 4208 CPU with 16 cores (32 threads) and 512 GB RAM.
\section{Hyperparameters}
We selected the hyperparameter $\lambda$ from the following set: $\lambda \in L=\{0, 0.0001, 0.0005, 0.001, 0.005, 0.01, 0.02,$ $0.04, 0.06, 0.08, 0.1, 0.5, 0.9, 1.0001 \}$.
Figure \ref{fig:lambda} illustrates the time decay function  $\Delta_\lambda(t,k)=2^{\lambda(k-t)}$ for these values.
Further, the hyperparameter $\alpha$ was chosen from the set: $\alpha \in A=\{0, 0.00001, 0.0001, 0.001, 0.01, 0.1,$ $0.5, 0.9, 0.99, 0.999, 0.9999, 0.99999, 1\}$.

To assess the impact of hyperparameter values on prediction scores, we stipulate values for $\lambda$ and $\alpha$ across all relations and show the prediction scores for different values of $\lambda$ and $\alpha$. 
Table~\ref{table:paramvalues} displays the values for $\alpha$ and $\lambda$, selected based on the validation MRR.
Furthermore, Table~\ref{table:paramvalueslambda} demonstrates how $\lambda$ influences the test MRR for the \srb ($\psi_\Delta$) on ICEWS14. 
To analyse the influence of $\alpha$ on the \rb, we set $\lambda=0.04$, which corresponds to the value that yielded the best performance on ICEWS14 for $\psi_\Delta$. 
Table \ref{table:paramvaluesalpha} presents the test MRR on ICEWS14 for different values of $\alpha$ for the \rb $\psi_{\Delta_{\lambda=0.04}}\xi$.

Table~\ref{table:resultsperlambda} presents the test MRR for the \srb $\psi$ for selected time decay settings on all datasets. We display results for $\lambda = \{0, 0.1, 1.0001\}$ stipulated for all relations, and values for $\lambda_r(\texttt{per rel)}$, i.e., $\lambda$ selected per relation based on validation MRR. 
From Proposition~3, we know that $\psi_{\Delta_{\lambda=0}}$ and $\psi_1$ are ranking equivalent, i.e. $\psi_{\Delta_{\lambda=0}} \Leftrightarrow \psi_1$. %where we have no time decay. 
Further, we know from Proposition~2 that $\psi_{\Delta_{\lambda=1.0001}} \Leftrightarrow \phi_\Delta$.
 % note: selected on a per dataset basis  based on validation MRRs.

Further, to understand the impact of the \rrb ($\xi$) on the combined baseline, Figure~\ref{fig:xipsi} presents a comparative analysis of the MRR of strict, relaxed, and combined baseline across individual relations within the YAGO dataset. For two relations hasWonPrize (tail) and diedIn (tail), the \rrb achieves significantly better results than the \srb. Remarkably, the \rb consistently demonstrates performance equal to or slightly better than the best-performing individual baseline across all relations examined. This observation underscores the effectiveness of the combined baseline approach and shows the benefit of selecting the value of $\alpha$ per relation. % as it consistently matches or even outperforms the top-performing individual baselines for each relation. 

\begin{figure}[t]
    \centering
    \includegraphics[width=.99\columnwidth]{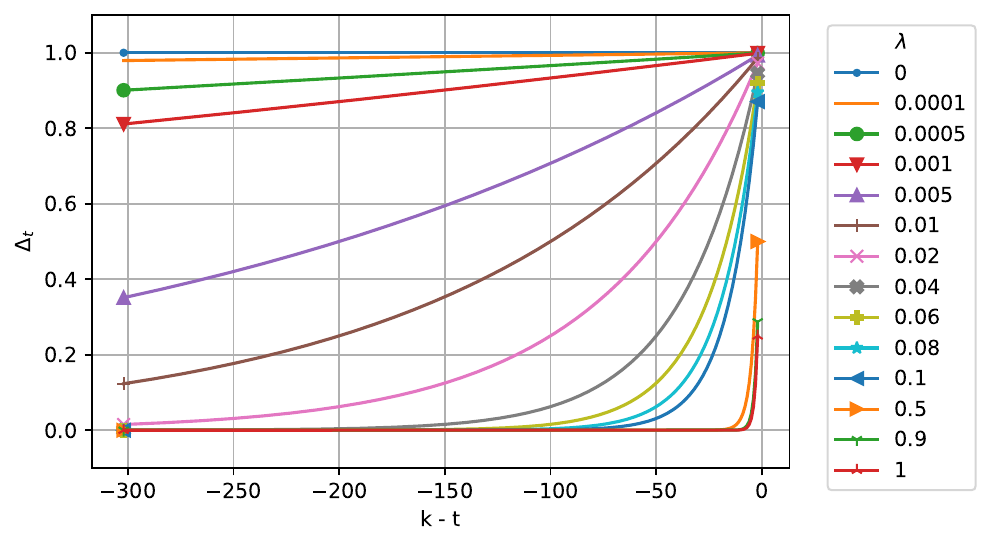}
    \caption{The time decay function $\Delta_\lambda(t,k)=2^{\lambda(k-t)}$ for different values of $\lambda$. $k-t$ represents the distance between the query timestep $t$ and the timestep of last occurence $k$.}
    \label{fig:lambda}
\end{figure}

\begin{figure}[t]
    \centering
    \includegraphics[width=.99\columnwidth]{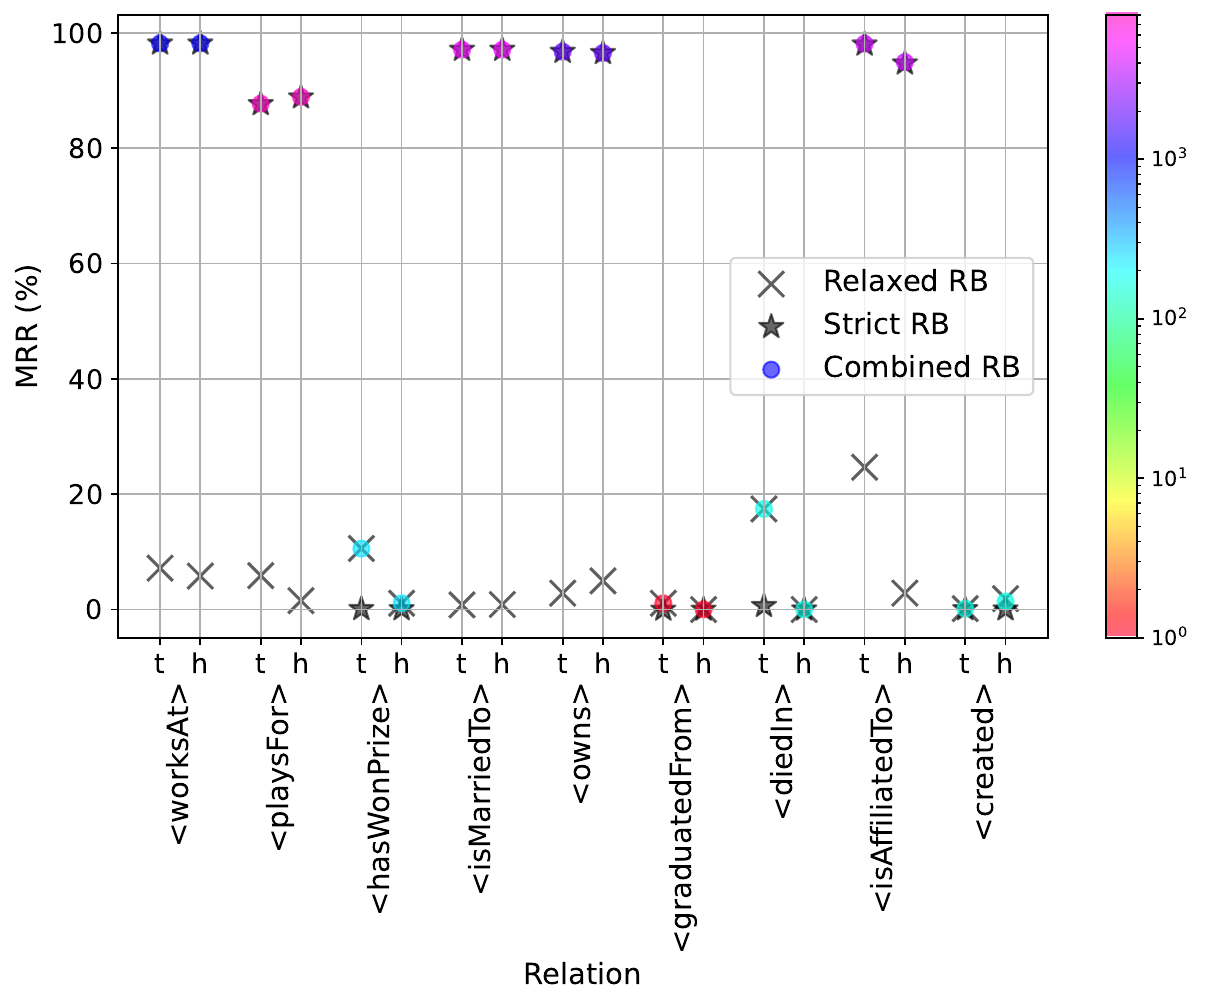}
    \caption{Test MRRs for the \rrb (cross), \srb (star), and \rb (dot) for each relation and direction (“t” means tail and “h” head, respectively) for YAGO. Colors indicate the number of queries for relation and its direction in the test set. }
    \label{fig:xipsi}
\end{figure}

\setlength{\tabcolsep}{5pt}
\begin{table*} 

%\scriptsize
\centering
\begin{tabular}{l|r|r|r|r|r}
\toprule
            & {GDELT} & {YAGO}      & {WIKI}    & {ICEWS14} & {ICEWS18} \\
\midrule
$\lambda$   & 0.01   & 1.0001      & 1.0001    & 0.02      & 0.02    \\
$\alpha$    & 0.99    & 0.99         & 0.99999   & 0.999    & 0.99     \\ % updated 2.1.2024
% $\lambda$   & 0.005   & 1.0001      & 1.0001    & 0.02      & 0.01    \\
% $\alpha$    & 0.99    & 0.5         & 0.99999   & 0.9999    & 0.99     \\
\bottomrule
  \end{tabular}
  \caption{Values for parameters $\lambda$ and $\alpha$ that have been selected per dataset when stipulating values for $\lambda$ and $\alpha$ across all relations.}
\label{table:paramvalues}
\end{table*}

\setlength{\tabcolsep}{5pt}
\begin{table*} 
%\scriptsize
\centering
\begin{tabular}{l|r|r|r|r|r|r|r|r|r|r|r|r|r|r}
\toprule
%\multicolumn{14}{l}{ $\psi_\Delta$ }    \\
%\midrule 
% \begin{tabular}{lllllllllllllllllllll}
$\lambda$  & 0         & 0.0001    & 0.0005    & 0.001     & 0.005     & 0.01      & 0.02      & 0.04      & 0.06      & 0.08      & 0.1       & 0.5       & 0.9       & 1.0001     \\
 MRR & 34.4     & 35.3    & 35.3     & 35.3     & 35.6     & 35.7     & 35.9     & 36.0     & 36.0     & 35.9     & 35.5     & 30.3     & 27.9     & 27.5     \\ %updated on 22.12. 
\bottomrule
  \end{tabular}
  \caption{Test MRR for the \srb ($\psi_\Delta$) for different values of $\lambda$. Example for dataset ICEWS14.}
\label{table:paramvalueslambda}
\end{table*}
\setlength{\tabcolsep}{5pt}
\begin{table*} 
%\scriptsize
\centering
\begin{tabular}{l|r|r|r|r|r|r|r|r|r|r|r|r|r}
\toprule
$\alpha$  &0         & 1.00E-05  & 0.0001    & 0.001     & 0.01      & 0.1       & 0.5       & 0.9       & 0.99      & 0.999     & 0.9999    & 0.99999   & 1        \\ % & -1     \\   %& -2   \\
MRR  & 14.4      & 14.6     & 14.6     & 14.6    & 14.8     & 17.5    & 27.0     & 34.7    & 35.9     & 36.6    & 37.1     & 37.2      & 37.2   \\ %   & 36.64   \\  %& 37.19 \\ % 22.12.
% updated 22.12.
\bottomrule
  \end{tabular}
  \caption{Test MRR for the \rb ($\psi_{\Delta_{\lambda=0.04}}\xi$) for different values of $\alpha$. Example for dataset ICEWS14.}
\label{table:paramvaluesalpha}
\end{table*}
\setlength{\tabcolsep}{5pt}
\begin{table*} 
%\scriptsize
\centering
\begin{tabular}{l|rr|rr|rr|rr|rr}
\toprule
& \multicolumn{2}{c|}{GDELT} & \multicolumn{2}{c|}{YAGO} & \multicolumn{2}{c|}{WIKI} & \multicolumn{2}{c|}{ICEWS14} & \multicolumn{2}{c}{ICEWS18} \\
\midrule
		                                      & MRR  & H@10 & MRR  & H@10 & MRR  & H@10 & MRR & H@10 & MRR & H@10  \\
\midrule
$\psi_{\Delta_{\lambda=0}} \Leftrightarrow \psi_{1}$         & 20.8 & 35.3 & 81.6 & 90.9 & 68.1 & 83.5 & 34.4 & 47.2 & 26.2 & 40.3 \\ %updated 22.12. baselinepsi_singlestep_0.0_1.0_1.0
$\psi_{\Delta_{\lambda=0.1}}$                                & 19.5 & 31.3 & 85.7 & 92.3 & 73.7 & 85.6 & 35.5 & 47.8 & 26.8 & 40.4 \\ %updated 22.12.  baselinepsi_singlestep_0.1_1.0_1.0
$\psi_{\Delta_{\lambda=1.0001}} \Leftrightarrow  \phi_{\Delta}$   & 12.1 & 18.3 & 90.7 & 92.8 & 81.6 & 87.0 & 27.5 & 33.8 & 21.0 & 29.9 \\  %updated 22.12. baselinepsi_singlestep_1.0001_1.0_1.0
$\psi_{\Delta_{\lambda_r (\texttt{per rel})}}$          & 23.7 & 38.3 & 90.7 & 92.8 & 81.6 & 87.0 & 36.3 & 48.4 & 27.8 & 41.4 \\ % update 22.12. baselinepsi_singlestep_-1_-1_0.0001 and baselinepsi_singlestep_-1_-1_1.0 (same configuration)
\bottomrule
  \end{tabular}
  \caption{Experimental results for single-step prediction on the \srb $\psi$ for different time decay settings, i.e. for different values of~$\lambda$.}
\label{table:resultsperlambda}
\end{table*}

\section{Results for Multi-step Prediction}
Multi-step prediction involves forecasting multiple future timesteps at once. In this setting, the model predicts all timesteps from the test set without having access to any ground truth information in between. Multi-step prediction presents a greater challenge because the model relies solely on its own forecasts, leading to an accumulation of uncertainty as the number of forecasted timesteps increases. \cite{gastinger2023eval}

Table \ref{table:results_multistep} shows the test results (MRR and Hits@10) for all datasets for the methods from related work that run in multi-step setting, as well as the \rrb ($\xi$), the \srb ($\psi_{\Delta}$), and the \rb ($\psi_{\Delta}\xi$). We obtain the results for related work following the evaluation protocol in \cite{gastinger2023eval}. The hyperparameter values for our baselines have been selected for each relation following the same procedure as described for the single-step setting.
\setlength{\tabcolsep}{5pt}
\begin{table*} 
%\scriptsize
\centering
\begin{tabular}{l|rr|rr|rr|rr|rr}
\toprule
& \multicolumn{2}{c|}{GDELT} & \multicolumn{2}{c|}{YAGO} & \multicolumn{2}{c|}{WIKI} & \multicolumn{2}{c|}{ICEWS14} & \multicolumn{2}{c}{ICEWS18} \\
\midrule
		                  & MRR  & H@10 & MRR  & H@10 & MRR  & H@10 & MRR & H@10 & MRR & H@10  \\
\midrule
RE-GCN                                                                     & 19.6          & 33.6          & 75.4          & 81.7          & 62.7          & 67.9          & \textbf{37.8} & \textbf{57.5} & \textbf{29.0} & \textbf{47.5} \\
RE-Net                                                                     & \textbf{19.7} & \textbf{33.9} & 58.2          & 66.3          & 49.5          & 53.0          & 37.0          & 54.9          & 27.9          & 46.2          \\
CyGNet                                                                     & 19.1          & 33.1          & 69.0          & 83.4          & 58.3          & 67.6          & 36.1          & 54.5          & 26.0          & 44.4          \\
TLogic                                                                     & 17.7          & 30.3          & 66.9          & 71.6          & 64.0          & 68.2          & 35.5          & 53.1          & 24.0          & 41.2          \\
\midrule
$\xi$             & 14.1          & 23.4          & 5.1           & 10.5          & 14.0          & 24.7          & 14.1          & 27.8          & 11.6          & 21.8          \\
$\psi_\Delta$           & 18.1          & 30.4          & 81.4          & 84.2          & 63.7          & 68.2          & 30.1          & 40.8          & 23.4          & 35.8          \\
$\psi_\Delta\xi$   & 19.2          & 32.5          & \textbf{81.7} & \textbf{84.6} & \textbf{64.3} & \textbf{69.0} & 31.7          & 45.4          & 24.6          & 38.6     \\    

\bottomrule
  \end{tabular}
  \caption{Experimental results for multi-step prediction.
}
\label{table:results_multistep}
\end{table*}

Overall, the scores for multi-step prediction are lower than those for single-step prediction, aligning with expectations. Furthermore, the results reveal a consistent pattern with the results obtained in single-step prediction. In comparison to related work, the \rb demonstrates superior performance in two out of the five datasets (YAGO and WIKI) and ranks third in performance for a third dataset (GDELT). For ICEWS14 and ICEWS18, the majority of methods from related work outperform the \rb, yielding better results.

\section{Runtime}
All baselines run on CPU; we use an Intel Xeon Silver (2.10GHz) 4208 CPU with 16 cores (32 threads) and 512 GB RAM.
The overall runtime is linear in the size of the dataset times the number of different hyperparameter settings, no matter the number of relations.
For each relation $r$, we tune the hyper-parameter values of $\lambda_r,\alpha_r$ on the subset of quadruples with relation $r$, which is a strict subset of the total quadruples. This is possible because relations are independent from each other.
Thus, for each hyper-parameter $\lambda_r,\alpha_r$ to be tuned, the complexity is linear in the number of quadruples of that specific relation times the number of values to try.

In Table~\ref{tab:run_rbas} we report total runtimes required for our baseline (to perform all steps, i.e. data loading, hyperparameter selection, and testing). In Table~\ref{tab:all}, as an example, we compare this number for ICEWS14 to time spent to perform all steps except hyperparameter tuning for the other methods considered in Section 5.2 (thus ignoring hyperparameter tuning altogether).
Despite performing hyperparameter selection, we need 20x less time than the fastest related method to get the final scores. 
    \begin{table}[]
        \centering
        \begin{tabular}{l|l|l|l|l}
        \toprule
            ICEWS14 & ICEWS18 & GDELT & YAGO & WIKI \\
            728 s & 6758 s & 22812 s& 778 s & 9215 s \\
        \bottomrule
        \end{tabular}
        \caption{Runtime including hyperparameter selection and testing for the Combined Recurrency Baseline $\psi_\Delta\xi$.}
        \label{tab:run_rbas}
    \end{table}
    \begin{table}[]
        \centering
        
        \begin{tabular}{l|l|l|l|l}
        \toprule
            $\psi_\Delta\xi$ & RE-GCN    & CEN   & xERTE & TLogic \\
            728 s         & 31052 s   & 14535 s & 51212 s & 15212 s \\
            %4h 2min 15 sek
        \bottomrule
        \end{tabular}
        \caption{Total Runtime on ICEWS14 for $\psi_\Delta\xi$ and the methods considered in Section 5.2 of the main paper. Total runtime means time to perform all steps, i.e. data loading, hyperparameter selection, and testing for $\psi_\Delta\xi$ and all steps except hyperparameter tuning for the other methods (thus ignoring hyperparameter tuning altogether). TLogic and $\psi_\Delta\xi$ run on CPU, % (Xeon Silver (2.10GHz) 4208 CPU, 16 cores (32 threads), 512 GB RAM), 
        the others on GPU.} % (GeForce RTX 2080 (12 GB)).} %, including all steps (e.g. preprocessing, training, testing, evaluation.)}
        \label{tab:all}
    \end{table}

\section{Additional Information on Related Work}
\paragraph{TRKG} Note on results for TRKG: We found that the authors of TRKG \cite{Kiran2023TRKG} compute their results (MRR and Hits@1,3,10) on the computation protocol "best". If there are multiple triples in the candidate set with the same score from the model, this protocol assigns the lowest rank, i.e. the best score, to the ground truth triple. As reported in \cite{Sun2020reevaluation}, this is an unfair evaluation protocol. Thus, we rerun the experiments for TRKG following the evaluation protocol introduced by \cite{gastinger2023eval}, who compute the ranks based on the "random" computation protocol. This explains the drop in result scores from the original TRKG paper as compared to our table.

\section{Additional Information on Datasets}
In the following we provide additional information on the datasets that we use for our experiments. For each dataset we use the version provided by~\cite{Li2021regcn} and~\cite{gastinger2023eval}.
% Researchers in the field of TKG Forecasting utilize several datasets:
\begin{description}   
\item{ICEWS Datasets:} ICEWS14 ~\cite{GarciaDuran2018ICEWS14} and ICEWS18~\cite{Jin2019oldrenet} are derived from the Integrated Crisis Early Warning System (ICEWS)~\cite{Boschee2015}, covering different time spans (for the years 2014 and 2018). ICEWS provides event data on various global events such as conflicts, protests, and diplomatic relations.

\item{GDELT:} The Global Database of Events, Language, and Tone (GDELT)~\cite{Leetaru2013GDELT} provides a comprehensive collection of global events derived from news articles and other sources. It covers a broad range of events, including political events, conflicts, and societal movements, spanning various geographic regions and time periods.

\item{YAGO and WIKI:} YAGO~\cite{Mahdisoltani2015YAGO} offers structured data regarding entities, facts, and their relationships. The WIKI dataset is extracted from Wikidata~\cite{vrandevcic2014wiki} and has first been preprocessed to contain temporal information by~\cite{Leblay2018WIKI}. % and 
We use versions of YAGO and WIKI that have further been preprocessed according to \cite{Jin2019oldrenet}, who formulate temporal information in quadruples and remove noisy events of early years (before 1786 for WIKI and 1830 for YAGO).

\end{description}
